# Supplementary material for: Multi-Fidelity Flow Matching: Cascaded Refinement of PDE Solutions
Source: arXiv:2605.16118 source file (2026-05-15)
Supplement: Supplementary file 1 [file F_error_visualization.tex]

\section{Predictive-uncertainty: full metric table and error-field visualizations}
\label{app:uq-tables-and-vis}

\subsection{Full UQ metric table}
\label{app:uq-table}

\begin{table}[h]
\centering
\small
\caption{Predictive-uncertainty metrics on three representative benchmarks. \textsc{MFFM (cascade)} draws the source from the calibrated $\N(0, \Sgmd)$. \textsc{MFFM (iid noise)} replaces $\Sgmd$ at each cascade level with $\bar{\sigma}^2 \mathbf{I}$, the isotropic noise of matched average variance, and re-runs inference on the same trained networks; this isolates the source-distribution choice. \textsc{PDE-Refiner} is run with $K = 4$ refinement steps and $K = 50$ posterior samples. Coverage is at nominal $90\%$ (ideal $0.90$); cal-err averages $\abs{\text{nominal} - \text{observed}}$ over $10$ levels in $[0.1, 0.95]$ (lower is better); spread/RMSE close to $1$ indicates correct uncertainty magnitude; $\rho(\sigma, \abs{\mathrm{err}})$ is the per-pixel Pearson correlation between predicted standard deviation and absolute error. Cells marked \plh{xxx} are placeholders.}
\label{tab:uq}
\setlength{\tabcolsep}{4pt}
\begin{tabular}{llccccccc}
\toprule
Benchmark & Method & NRMSE & CRPS & Cov$_{90}$ & Sharp$_{90}$ & spread / RMSE & $\rho(\sigma, \abs{\mathrm{err}})$ & cal-err \\
\midrule
\multirow{3}{*}{SW}
  & PDE-Refiner            & \plh{xxx} & \plh{xxx} & \plh{xxx}  & \plh{xxx} & \plh{xxx} & \plh{xxx} & \plh{xxx} \\
  & MFFM (iid noise)       & \plh{xxx} & \plh{xxx}& \plh{xxx}  & \plh{xxx} & \plh{xxx} & \plh{xxx} & \plh{xxx} \\
  & \textbf{MFFM (calib.)} & \plh{xxx} & \plh{xxx}& \plh{xxx}  & \plh{xxx} & \plh{xxx} & \plh{xxx} & \plh{xxx} \\
\midrule
\multirow{3}{*}{DR}
  & PDE-Refiner            & \plh{xxx} & \plh{xxx} & \plh{xxx}  & \plh{xxx} & \plh{xxx} & \plh{xxx} & \plh{xxx} \\
  & MFFM (iid noise)       & \plh{xxx} & \plh{xxx} & \plh{xxx}  & \plh{xxx} & \plh{xxx} & \plh{xxx} & \plh{xxx} \\
  & \textbf{MFFM (calib.)} & \plh{xxx} & \plh{xxx} & \plh{xxx}  & \plh{xxx} & \plh{xxx} & \plh{xxx} & \plh{xxx} \\
\midrule
\multirow{3}{*}{Shear-P}
  & PDE-Refiner            & \plh{xxx} & \plh{xxx} & \plh{xxx}  & \plh{xxx} & \plh{xxx} & \plh{xxx} & \plh{xxx} \\
  & MFFM (iid noise)       & \plh{xxx} & \plh{xxx} & \plh{xxx}  & \plh{xxx} & \plh{xxx} & \plh{xxx} & \plh{xxx} \\
  & \textbf{MFFM (calib.)} & \plh{xxx} & \plh{xxx} & \plh{xxx}  & \plh{xxx} & \plh{xxx} & \plh{xxx} & \plh{xxx} \\
\bottomrule
\end{tabular}
\end{table}
